# Supplementary material for: Triformer: Triangular, Variable-Specific Attentions for Long Sequence Multivariate Time Series Forecasting--Full Version
Source: arXiv:2204.13767 source file (2022-04-28)
Supplement: Supplementary file 1 [file appendix.tex]

\typeout{IJCAI--22 Multiple authors example}

% These are the instructions for authors for IJCAI-22.

\documentclass{article}
\pdfpagewidth=8.5in
\pdfpageheight=11in
% The file ijcai22.sty is NOT the same as previous years'
\usepackage{ijcai22}

% Use the postscript times font!
\usepackage{times}

\usepackage{soul}
\usepackage{url}
\usepackage[hidelinks]{hyperref}
\usepackage[utf8]{inputenc}
\usepackage[small]{caption}
\usepackage{graphicx}
\usepackage{amsmath}
\usepackage{booktabs}
\urlstyle{same}

% ADDED BY US

\usepackage[nointegrals]{wasysym}
\usepackage{xcolor}
\usepackage{multirow}
\usepackage{amssymb}
\usepackage{subcaption}
\usepackage{stackengine}
\usepackage{float}
\usepackage{graphicx}
\usepackage{booktabs}
\usepackage{times}
\usepackage{amsmath}
\usepackage{wrapfig}
\usepackage{pbox}
\usepackage[export]{adjustbox}
\usepackage[normalem]{ulem}
% \captionsetup{justification=raggedright,singlelinecheck=false}

% \usepackage{booktabs}

% \pagenumbering{roman}

\pagenumbering{arabic}

\frenchspacing
\setlength{\pdfpagewidth}{8.5in}
\setlength{\pdfpageheight}{11in}
\pdfinfo{
/Title (Insert Your Title Here)
/Author (Put All Your Authors Here, Separated by Commas)}
\setcounter{secnumdepth}{0}

\begin{document}

\section{Appendix}

\subsection{Additional Related Work}

\bibliographystyle{named}
\bibliography{references}
\end{document}
